# Supplementary material for: Observation of the dominant spin-triplet supercurrent in Josephson spin valves with strong Ni ferromagnets
Source: arXiv:1912.08587 source file (2019-12-18)
Supplement: Supplementary file 1 [file Suppl_Kapran_PRXv1.pdf]

Observation of the dominant spin-triplet supercurrent in Josephson spin valves with strong Ni ferromagnets
(Kapran, et al.)

## SUPPLEMENTARY MATERIAL

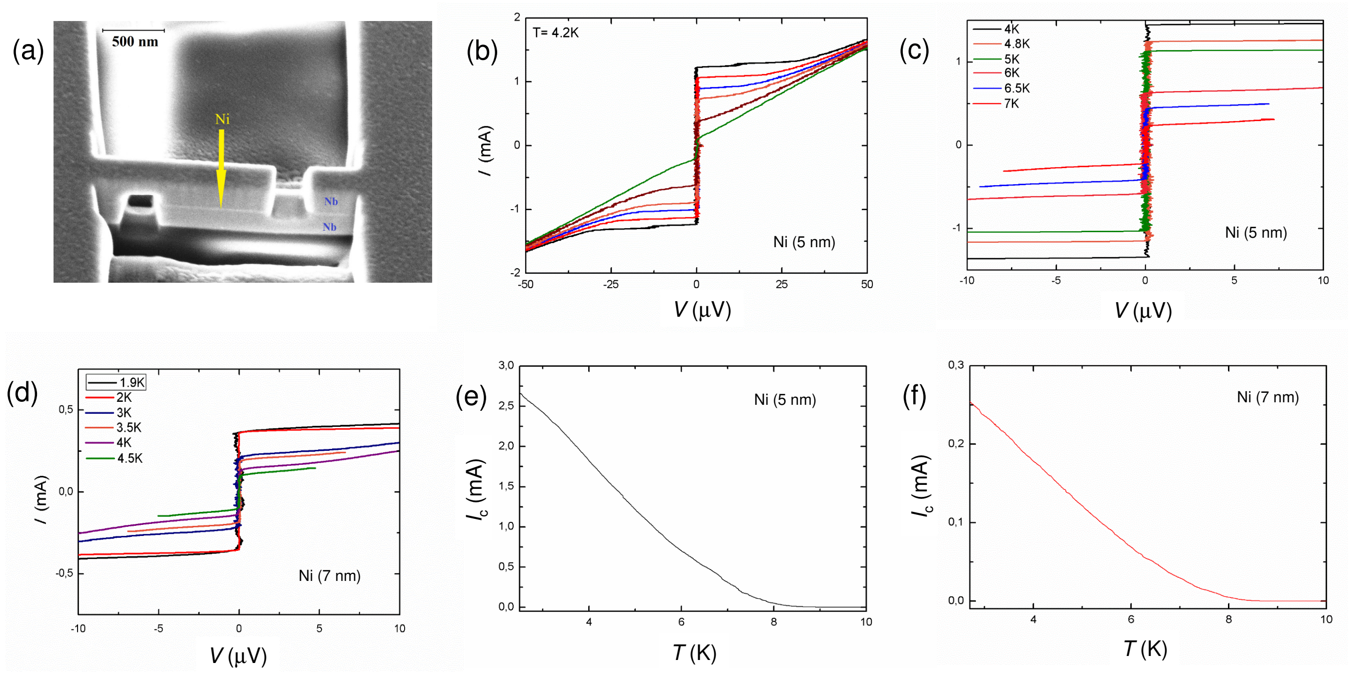


Supplementary Figure 1. **Properties of Nb/Ni/Nb SFS junctions.** (a) SEM image of a studied SFS junction. (b) $I$-$V$ characteristics for a junction with Ni(5 nm) at different magnetic field and $T = 4.2$ K. (c) $I$-$V$ characteristics of the same junction with Ni(5 nm) at different temperatures and $H = 0$. (d) $I$-$V$ characteristics of a junction with Ni(7 nm) at different temperatures and $H = 0$. (e) and (f) Temperature dependencies of the critical current for junctions with (e) Ni(5 nm) and (f) Ni (7 nm).

## SUPPLEMENTARY NOTES

### Supplementary Note 1. Properties of Nb/Ni/Nb SFS junctiosn

Supplementary Figure 1 shows a SEM image of one of the studied Nb/Ni/Nb SFS junctions with Ni(5 nm) and sizes $237 \times 942$ nm$^2$. Junctions were made in a similar manner, had similar sizes and geometries as JSV's. Suppl. Fig. 1 (b) show $I$-$V$ characteristics of the same junction with 5 nm Ni thickness at different magnetic fields $H \sim$ 0-1 kOe and $T = 4.2$ K. It is seen that the characteristic voltage $I_c R_n \sim 50\mu$V is rather high for SFS junctions, indicating large critical current through a thin Ni interlayer. It is seen that the critical current is suppressed by magnetic fields, which together with regular Fraunhofer-type modulation $I_c(H)$, see Fig. 2, indicates good uniformity of Ni interlayer in the junction.

Suppl. Figs 1 (c) and (d) show temperature evolutions of $I$-$V$ curves, and Suppl. Figs 1 (e) and (f) show temperature dependencies of $I_c$ for junctions with (c,e) 5 nm and (d,f) 7 nm ($220 \times 1000$ nm$^2$) Ni layer thicknesses, respectively.

### Supplementary Note 2. Determination of the critical current

Critical currents were determined automatically upon sweeping external parameters (field, or temperature). For this $I$-$V$ characteristics were recorded and several characteristics were analyzed simultaneously. We used three methods for determination of $I_c$. Two methods involve on-flight analysis of dc $I$-$V$ characteristics. Supplementary Figure 2 (a)

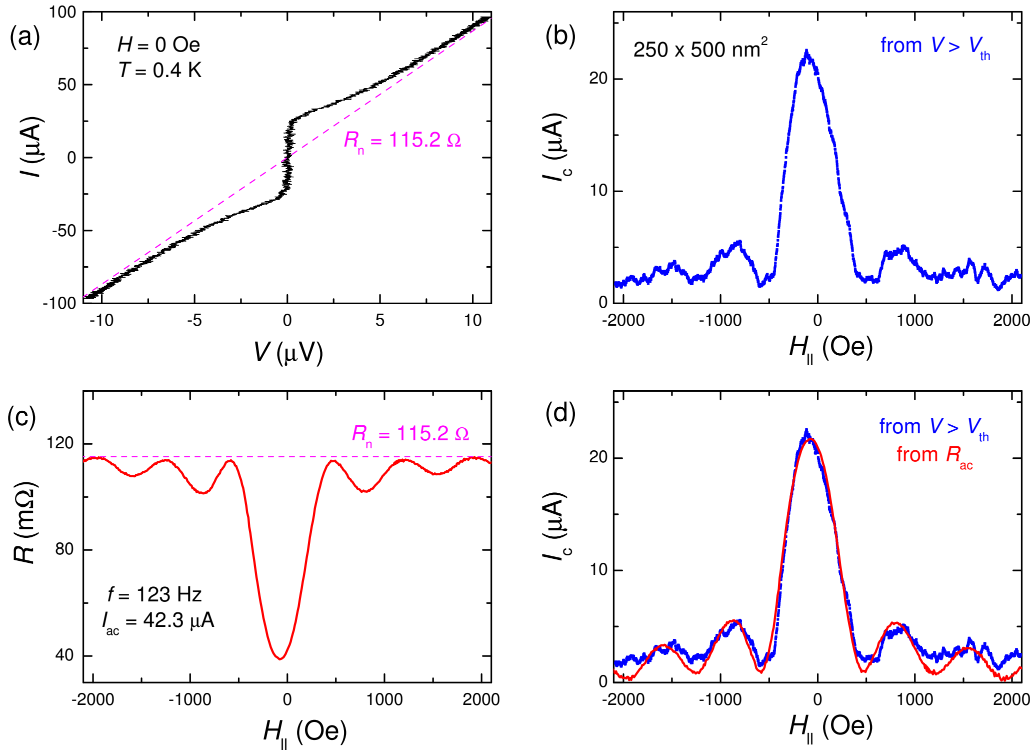


Supplementary Figure 2. **Clarification of determination of the critical current.** (a) Current-Voltage characteristics of a device with sizes $250 \times 500$ nm$^2$ at zero field and $T \simeq 0.4$ K. The dashed line indicates normal resistance $R_n = 115.2$ m$\Omega$. (b) Measured modulation of the critical current, determined by the threshold voltage criterium $V > V_{th}$, versus magnetic field along the long side of the device. The excess noise is caused by the small characteristic voltage $I_c R_n \sim 2.6$ $\mu$V, due to which the threshold voltage $V_{th} \sim 0.25$ $\mu$V is close to the dc-voltage noise level. (c) Measured (lock-in) ac-resistance at $f = 123$ Hz and ac-current amplitude $I_{ac} \simeq 30$ $\mu$A vs. magnetic field. Minima/maxima of $R(H)$ occur at maxima/minima of $I_c(H)$. The horizontal dashed line indicates $R_n$ level. It is seen that at maxima $R(H) = R_n$, which indicates that $I_c = 0$ at those points. (d) Comparison of $I_c(H)$ patterns obtained from using the voltage threshold criterium (blue) and recalculated from $R_{ac}$ (red). Both curves were measured simultaneously for the same downward field sweep. Apparently, the two measurement techniques are equivalent, however, the lock-in measurement is less noisy and correctly reproduces $I_c(H)$ modulation at high fields where the threshold method fails because $I_c(H) < V_{th}/R_n$.

shows an example of a typical $I$-$V$. From such analysis we can determine $I_c$ by either finding the point of deviation from zero resistance, when the voltage becomes larger than some threshold voltage $V_{th}$, or by finding the inflection point at the $I$-$V$'s. However, due to significant $1/f$ noise in dc-measurements in combination with small resistances (few tens of m$\Omega$) and small characteristic voltages $I_c R_n \sim \mu$V) of studied devices, dc-characteristics are rather noisy. This is demonstrated in the Supplementary Figure 2 (b), which represents $I_c(H)$ obtained for a downward field sweep using the threshold voltage method with $V_{th} \simeq 0.25$ $\mu$V. Furthermore, this method can not measure critical currents smaller than $V_{th}/R_n$, which does not allow confident determination of $I_c$ at high fields and at zeroes of $I_c$ at integer flux quanta in the device, see Supplementary Fig. 2 (b).

Much more accurate determination of $I_c$ can be made via lock-in measurement of ac-resistances at fairly high frequencies, $f > 100$ Hz, at which noise is several orders of magnitude lower than in dc-measurements. Supplementary Fig. 2 (c) represents ac-resistance versus field, measured at $f = 123$ Hz with the ac-current amplitude slightly larger than the maximum critical current. The measurement is done during the same downward field sweep as in Suppl. Fig. 2(b). Apparently, $R(H)$ shows modulation, which is inverse (flipped) with respect to $I_c(H)$ pattern. Minima/maxima of $R(H)$ correspond to maxima/minima of $I_c$. Thus, $I_c(H)$ is encoded and can be extracted from $R(H)$ modulation, measured at low bias $I_{ac} \gtrsim I_{c0}$.

Within the Resistively Shunted Junction (RSJ) model, the $I$-$V$ has a shape.

$$V = R_n \sqrt{I^2 - I_c^2}. \tag{1}$$

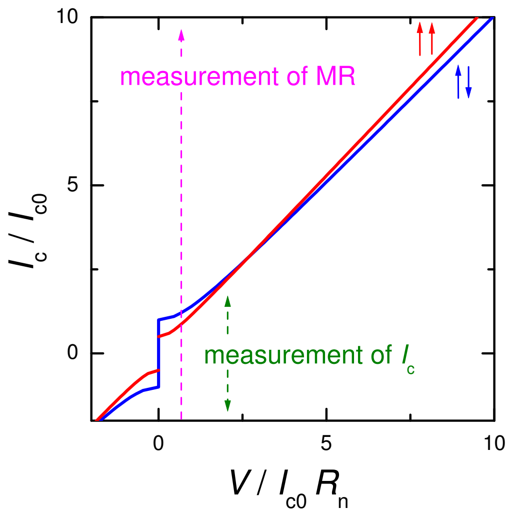


Supplementary Figure 3. **Clarification of lock-in responses of a Josephson spin valve at low and high ac-bias.** A sketch of $I$-$V$ characteristics of a JSV in antiparallel (blue, high $R_n$) and parallel (red, low $R_n$) orientations of magnetizations. Dashed vertical arrows indicate two ways of probing JSV's by lock-in measurements with low (olive) and high (magenta) bias currents. The low bias ac-resistance $R(H)$, measured with $I_{\mathrm{ac}} \gtrsim I_{\mathrm{c0}}$ in a strongly non-linear part of the $I$-$V$, reflects Fraunhofer modulation of $I_{\mathrm{c}}(H)$ and is used for determination of $I_c$. High bias resistance $I_{\mathrm{ac}} \gg I_{\mathrm{c0}}$, measured in the linear part of the $I$-$V$, represents the spin-valve magnetoresistance (MR) that depends on relative orientation of two ferromagnetic layers.

Consequently, $I_c = I\left(1 - (R_{dc}/R_n)^2\right)^{0.5}$, where $R_{dc} = V/I$ is the dc-resistance. This formula, however, can not be directly applied for conversion of lock-in resistance $R_{ac}$ into $I_c$ because due to nonlinearity of $I$-$V$ curves $R_{ac} \neq R_{dc}$ and because the shape of the $I$-$V$ may deviate from the RSJ model. Therefore, we use a more general fitting function:

$$I_c = I_{ac}\left[1 - \left(\frac{R_{ac}}{R_n}\right)^{\alpha}\right]^{\beta}, \tag{2}$$

with constant exponents $\alpha > 1$ and $\beta < 1$. Using $\alpha$ and $\beta$ as fitting parameters we fit Eq. 2 to $I_c(H)$ obtained from analysis of dc $I$-$V$ curves. Red line in the Supplementary Fig. 2 (d) demonstrates a result of such fitting. Apparently, it not only properly reproduces $I_c(H)$, but also significantly reduces noise and corrects an artifact of inaccurate dc-measurement of small critical currents $I_c < V_{th}/R_n$. Therefore, all $I_c(H)$ patterns, presented in the manuscript, were obtained from lock-in measurements. We want to emphasize that the conversion just flips the $R_{ac}(H)$ curve and does not change the symmetry or the basic shape of the curve, cf. Suppl. Figs. 2 (b) and (c). For example, it can not change a single-peak into a double peak, nor change relative amplitudes of consecutive maxima. Therefore, all the conclusions made in the manuscript could be obtained even without such a conversion, which just simplifies perception of the data.

### Supplementary Note 3. Measurement of spin-valve magnetoresistance

Supplementary Figure 3 shows a sketch of $I$-$V$ curves of a JSV in parallel (red) and antiparallel (blue) states. Orientation of the JSV affects both the critical current and the normal resistance $R_n$, which is larger in the antiparallel state. In the Supplementary Note 2 we described determination of $I_c$ from lock-in measurements of ac-resistance in a non-linear part of the $I$-$V$ at low bias currents $I_{ac} \gtrsim I_{c0}$. The corresponding low-bias current range is indicated by the olive vertical dashed arrows.

Determination of spin-valve magnetoresistance requires accurate measurements of the linear slope of $I$-$V$ curves far away from the critical current, i.e., measurements at large bias $I_{ac} \gg I_{c0}$, as indicated by the magenta dashed vertical arrow. Thus, lock-in measurements provide either critical current or spin-valve MR at low and high ac-amplitude, respectively.
